# Supplementary material for: Computation of drug solvation free energy in supercritical CO2: alternatives to all-atom computer simulations
Source: arXiv:2105.07240 source file (2021-05-15)
Supplement: Supplementary file 1 [file table_for_si.pdf]

ASP_Huang

| T, K | p^sat, Pa | v^s, m^3/mol | | T, K | p^sat, Pa | | | T, K | p^sat, Pa | | |
|---|---|---|---|---|---|---|---|---|---|---|---|
| 308,15 | 0,01 | 1,30E-04 | | 318,15 | 0,04 | | | 328,15 | 0,14 | | |

| P x10^5 Pa | delta_G kcal/mol | y m.f. | rho mol/m^3 | P x10^5 Pa | delta_G kcal/mol | y m.f. | rho mol/m^3 | P x10^5 Pa | delta_G kcal/mol | y m.f. | rho mol/m^3 |
|---|---|---|---|---|---|---|---|---|---|---|---|
| 120 | -7,52 | 8,90E-05 | 17430 | 120 | -6,72 | 7,20E-05 | 14945 | 120 | -5,88 | 6,30E-05 | 11464 |
| 150 | -7,61 | 1,12E-04 | 18520 | 150 | -7,12 | 1,39E-04 | 16859 | 150 | -6,46 | 1,37E-04 | 14849 |
| 172 | -7,61 | 1,22E-04 | 19090 | 172 | -7,22 | 1,75E-04 | 17687 | 172 | -6,63 | 1,82E-04 | 16085 |
| 185 | -7,61 | 1,29E-04 | 19376 | 185 | -7,27 | 1,95E-04 | 18077 | 185 | -6,77 | 2,34E-04 | 16626 |
| 200 | -7,59 | 1,33E-04 | 19671 | 200 | -7,29 | 2,12E-04 | 18466 | 200 | -6,86 | 2,77E-04 | 17146 |
| 215 | -7,60 | 1,42E-04 | 19938 | 215 | -7,30 | 2,28E-04 | 18808 | 215 | -6,85 | 2,86E-04 | 17588 |
| 230 | -7,57 | 1,45E-04 | 20182 | 230 | -7,28 | 2,34E-04 | 19113 | 230 | -6,85 | 3,03E-04 | 17973 |
| 250 | -7,54 | 1,51E-04 | 20478 | 250 | -7,29 | 2,58E-04 | 19476 | 250 | -6,89 | 3,47E-04 | 18420 |

ASP_Champeau

| T, K | p^sat, Pa | v^s, m^3/mol | | T, K | p^sat, Pa | | | T, K | p^sat, Pa | | |
|---|---|---|---|---|---|---|---|---|---|---|---|
| 313,15 | 0,02 | 1,30E-04 | | 328,15 | 0,14 | | | 353,15 | 2,34 | | |

| P x10^5 Pa | delta_G kcal/mol | y m.f. | rho mol/m^3 | P x10^5 Pa | delta_G kcal/mol | y m.f. | rho mol/m^3 | P x10^5 Pa | delta_G kcal/mol | y m.f. | rho mol/m^3 |
|---|---|---|---|---|---|---|---|---|---|---|---|
| 90 | -6,10 | 1,95E-05 | 10977 | 110 | -5,09 | 2,21E-05 | 9411 | 120 | -3,68 | 4,05E-05 | 6738 |
| 95 | -6,55 | 3,41E-05 | 13144 | 120 | -5,71 | 4,99E-05 | 11446 | 130 | -3,99 | 5,74E-05 | 7702 |
| 100 | -6,79 | 4,79E-05 | 14260 | 130 | -6,04 | 7,62E-05 | 12967 | 150 | -4,55 | 1,12E-04 | 9698 |
| 130 | -7,21 | 9,18E-05 | 16873 | 150 | -6,41 | 1,31E-04 | 14838 | 170 | -4,96 | 1,86E-04 | 11487 |
| 150 | -7,31 | 1,13E-04 | 17720 | 175 | -6,63 | 1,88E-04 | 16211 | 200 | -5,47 | 3,78E-04 | 13487 |
| 200 | -7,46 | 1,70E-04 | 19076 | 200 | -6,73 | 2,35E-04 | 17139 | 248 | -5,77 | 6,40E-04 | 15521 |
| 250 | -7,40 | 1,90E-04 | 19979 | 240 | -6,78 | 2,91E-04 | 18199 | 300 | -5,91 | 9,20E-04 | 16937 |
| 300 | -7,31 | 2,00E-04 | 20670 | 285 | -6,83 | 3,73E-04 | 19070 | | | | |
| 350 | -7,24 | 2,24E-04 | 21237 | | | | | | | | |

CBZ_Yamini

| T, K | p^sat, Pa | v^s, m^3/mol | | T, K | p^sat, Pa | | | T, K | p^sat, Pa | | |
|---|---|---|---|---|---|---|---|---|---|---|---|
| 308,15 | 2,49E-05 | 1,80E-04 | | 318,15 | 9,71E-05 | | | 328,15 | 3,49E-04 | | |

| P x10^5 Pa | delta_G kcal/mol | y m.f. | rho mol/m^3 | P x10^5 Pa | delta_G kcal/mol | y m.f. | rho mol/m^3 | P x10^5 Pa | delta_G kcal/mol | y m.f. | rho mol/m^3 |
|---|---|---|---|---|---|---|---|---|---|---|---|
| | | | | 122 | -8,78 | 6,00E-06 | 15175 | 122 | -7,65 | 3,00E-06 | 11864 |
| | | | | 152 | -8,91 | 8,00E-06 | 16973 | 152 | -8,23 | 7,00E-06 | 15018 |
| | | | | 182 | -9,01 | 1,10E-05 | 18013 | 182 | -8,39 | 1,00E-05 | 16534 |
| | | | | 213 | -9,10 | 1,50E-05 | 18782 | 213 | -8,47 | 1,30E-05 | 17552 |
| 243 | -9,33 | 1,10E-05 | 20393 | 243 | -9,07 | 1,70E-05 | 19370 | 243 | -8,61 | 1,90E-05 | 18287 |
| 274 | -9,31 | 1,30E-05 | 20812 | 274 | -9,06 | 2,00E-05 | 19875 | 274 | -8,65 | 2,40E-05 | 18898 |
| 304 | -9,24 | 1,40E-05 | 21170 | 304 | -9,00 | 2,20E-05 | 20297 | 304 | -8,64 | 2,80E-05 | 19395 |
| 334 | -9,16 | 1,50E-05 | 21491 | 334 | -8,94 | 2,40E-05 | 20669 | 334 | -8,63 | 3,30E-05 | 19826 |
| 355 | -9,12 | 1,60E-05 | 21698 | 355 | -8,95 | 2,80E-05 | 20906 | 355 | -8,61 | 3,60E-05 | 20097 |

IBU_Charoenchaitrakool

| T, K | p^sat, Pa | v^s, m^3/mol | | T, K | p^sat, Pa | | | T, K | p^sat, Pa | | |
|---|---|---|---|---|---|---|---|---|---|---|---|
| 308,15 | 8,09E-03 | 1,82E-04 | | 313,15 | 1,67E-02 | | | 318,15 | 3,35E-02 | | |
| P x10^5 Pa | delta_G kcal/mol | y m.f. | rho mol/m^3 | P x10^5 Pa | delta_G kcal/mol | y m.f. | rho mol/m^3 | P x10^5 Pa | delta_G kcal/mol | y m.f. | rho mol/m^3 |
| 80 | -6,99 | 5,30E-05 | 9523 | 95 | -8,30 | 5,85E-04 | 13179 | 85 | -5,11 | 1,15E-05 | 6403 |
| 85 | -8,62 | 5,43E-04 | 13909 | 120 | -9,18 | 2,32E-03 | 16309 | 90 | -5,76 | 2,80E-05 | 7669 |
| 90 | -9,02 | 9,95E-04 | 15045 | 140 | -9,32 | 3,18E-03 | 17343 | 95 | -6,11 | 4,10E-05 | 9420 |
| 100 | -9,21 | 1,35E-03 | 16197 | 170 | -9,47 | 4,67E-03 | 18357 | 100 | -7,48 | 3,10E-04 | 11321 |
| 110 | -9,37 | 1,81E-03 | 16904 | 200 | -9,59 | 6,80E-03 | 19082 | 110 | -7,98 | 6,02E-04 | 13705 |
| 120 | -9,44 | 2,13E-03 | 17430 | 220 | -9,49 | 6,49E-03 | 19478 | 120 | -8,20 | 8,37E-04 | 14945 |
| 130 | -9,51 | 2,50E-03 | 17853 | | | | | 140 | -8,51 | 1,44E-03 | 16371 |
| 140 | -9,46 | 2,43E-03 | 18210 | | | | | 170 | -8,58 | 1,82E-03 | 17622 |
| 150 | -9,49 | 2,68E-03 | 18520 | | | | | | | | |
| 160 | -9,57 | 3,23E-03 | 18795 | | | | | | | | |
| 170 | -9,64 | 3,82E-03 | 19043 | | | | | | | | |
| 180 | -9,59 | 3,78E-03 | 19269 | | | | | | | | |
| 200 | -9,59 | 4,23E-03 | 19671 | | | | | | | | |
| 210 | -9,55 | 4,23E-03 | 19852 | | | | | | | | |
| 220 | -9,54 | 4,41E-03 | 20022 | | | | | | | | |

IBU_Ardjmand_set_I

| T, K | p^sat, Pa | v^s, m^3/mol | | T, K | p^sat, Pa | | | T, K | p^sat, Pa | | |
|---|---|---|---|---|---|---|---|---|---|---|---|
| 308,15 | 4,95E-02 | 1,82E-04 | | 313,15 | 8,97E-02 | | | 318,15 | 1,60E-01 | | |
| P x10^5 Pa | delta_G kcal/mol | y m.f. | rho mol/m^3 | P x10^5 Pa | delta_G kcal/mol | y m.f. | rho mol/m^3 | P x10^5 Pa | delta_G kcal/mol | y m.f. | rho mol/m^3 |
| 80 | -5,77 | 4,28E-05 | 9912 | 90 | -6,49 | 1,98E-04 | 11196 | 80 | -4,04 | 1,15E-05 | 5496 |
| 85 | -7,48 | 5,11E-04 | 14033 | 95 | -7,24 | 5,73E-04 | 13282 | 85 | -4,68 | 2,80E-05 | 6433 |
| 90 | -7,85 | 9,03E-04 | 15119 | 100 | -7,45 | 7,66E-04 | 14354 | 90 | -5,02 | 4,10E-05 | 7722 |
| 95 | -7,99 | 1,12E-03 | 15768 | 105 | -7,83 | 1,39E-03 | 15056 | 95 | -5,75 | 1,09E-04 | 9509 |
| 100 | -8,07 | 1,29E-03 | 16243 | 110 | -7,91 | 1,60E-03 | 15578 | 100 | -6,50 | 3,10E-04 | 11419 |
| 105 | -8,14 | 1,47E-03 | 16622 | 115 | -8,09 | 2,14E-03 | 15996 | 105 | -6,97 | 6,02E-04 | 12821 |
| 110 | -8,23 | 1,71E-03 | 16940 | 120 | -8,12 | 2,29E-03 | 16346 | 110 | -7,20 | 8,37E-04 | 13768 |
| 115 | -8,24 | 1,78E-03 | 17216 | 125 | -8,28 | 3,02E-03 | 16648 | 115 | -7,56 | 1,44E-03 | 14455 |
| 120 | -8,37 | 2,27E-03 | 17460 | 130 | -8,32 | 3,26E-03 | 16915 | 120 | -7,70 | 1,82E-03 | 14990 |
| 125 | -8,41 | 2,47E-03 | 17680 | | | | | 125 | -7,87 | 2,38E-03 | 15428 |
| 130 | -8,45 | 2,71E-03 | 17880 | | | | | 130 | -7,98 | 2,84E-03 | 15798 |

IBU_Ardjmand_set_II

| T, K | p^sat, Pa | v^s, m^3/mol | | T, K | p^sat, Pa | | | T, K | p^sat, Pa | | |
|---|---|---|---|---|---|---|---|---|---|---|---|
| 308,15 | 3,43E-03 | 1,82E-04 | | 313,15 | 7,67E-03 | | | 318,15 | 1,69E-02 | | |
| P x10^5 Pa | delta_G kcal/mol | y m.f. | rho mol/m^3 | P x10^5 Pa | delta_G kcal/mol | y m.f. | rho mol/m^3 | P x10^5 Pa | delta_G kcal/mol | y m.f. | rho mol/m^3 |
| 80 | -7,42 | 4,28E-05 | 9912 | 90 | -8,04 | 1,98E-04 | 11196 | 80 | -5,48 | 1,15E-05 | 5496 |
| 85 | -9,13 | 5,11E-04 | 14033 | 95 | -8,78 | 5,73E-04 | 13282 | 85 | -6,12 | 2,80E-05 | 6433 |
| 90 | -9,50 | 9,03E-04 | 15119 | 100 | -8,99 | 7,66E-04 | 14354 | 90 | -6,45 | 4,10E-05 | 7722 |
| 95 | -9,64 | 1,12E-03 | 15768 | 105 | -9,37 | 1,39E-03 | 15056 | 95 | -7,18 | 1,09E-04 | 9509 |
| 100 | -9,72 | 1,29E-03 | 16243 | 110 | -9,46 | 1,60E-03 | 15578 | 100 | -7,94 | 3,10E-04 | 11419 |
| 105 | -9,79 | 1,47E-03 | 16622 | 115 | -9,63 | 2,14E-03 | 15996 | 105 | -8,41 | 6,02E-04 | 12821 |
| 110 | -9,87 | 1,71E-03 | 16940 | 120 | -9,67 | 2,29E-03 | 16346 | 110 | -8,64 | 8,37E-04 | 13768 |
| 115 | -9,89 | 1,78E-03 | 17216 | 125 | -9,83 | 3,02E-03 | 16648 | 115 | -8,99 | 1,44E-03 | 14455 |
| 120 | -10,02 | 2,27E-03 | 17460 | 130 | -9,86 | 3,26E-03 | 16915 | 120 | -9,14 | 1,82E-03 | 14990 |
| 125 | -10,06 | 2,47E-03 | 17680 | | | | | 125 | -9,31 | 2,38E-03 | 15428 |
| 130 | -10,10 | 2,71E-03 | 17880 | | | | | 130 | -9,41 | 2,84E-03 | 15798 |

IBU_Ardjmand_set_III

| T, K | p^sat, Pa | v^s, m^3/mol | | T, K | p^sat, Pa | | | T, K | p^sat, Pa | | |
|---|---|---|---|---|---|---|---|---|---|---|---|
| 308,15 | 8,09E-03 | 1,82E-04 | | 313,15 | 1,67E-02 | | | 318,15 | 3,35E-02 | | |
| P x10^5 Pa | delta_G kcal/mol | y m.f. | rho mol/m^3 | P x10^5 Pa | delta_G kcal/mol | y m.f. | rho mol/m^3 | P x10^5 Pa | delta_G kcal/mol | y m.f. | rho mol/m^3 |
| 80 | -6,88 | 4,28E-05 | 9912 | 90 | -7,54 | 1,98E-04 | 11196 | 80 | -5,03 | 1,15E-05 | 5496 |
| 85 | -8,59 | 5,11E-04 | 14033 | 95 | -8,29 | 5,73E-04 | 13282 | 85 | -5,67 | 2,80E-05 | 6433 |
| 90 | -8,96 | 9,03E-04 | 15119 | 100 | -8,49 | 7,66E-04 | 14354 | 90 | -6,01 | 4,10E-05 | 7722 |
| 95 | -9,10 | 1,12E-03 | 15768 | 105 | -8,87 | 1,39E-03 | 15056 | 95 | -6,73 | 1,09E-04 | 9509 |
| 100 | -9,18 | 1,29E-03 | 16243 | 110 | -8,96 | 1,60E-03 | 15578 | 100 | -7,49 | 3,10E-04 | 11419 |
| 105 | -9,25 | 1,47E-03 | 16622 | 115 | -9,14 | 2,14E-03 | 15996 | 105 | -7,96 | 6,02E-04 | 12821 |
| 110 | -9,33 | 1,71E-03 | 16940 | 120 | -9,17 | 2,29E-03 | 16346 | 110 | -8,19 | 8,37E-04 | 13768 |
| 115 | -9,35 | 1,78E-03 | 17216 | 125 | -9,33 | 3,02E-03 | 16648 | 115 | -8,54 | 1,44E-03 | 14455 |
| 120 | -9,48 | 2,27E-03 | 17460 | 130 | -9,37 | 3,26E-03 | 16915 | 120 | -8,69 | 1,82E-03 | 14990 |
| 125 | -9,52 | 2,47E-03 | 17680 | | | | | 125 | -8,86 | 2,38E-03 | 15428 |
| 130 | -9,56 | 2,71E-03 | 17880 | | | | | 130 | -8,96 | 2,84E-03 | 15798 |
